# Supplementary material for: The Effects of GitHub Copilot on Computing Students' Programming Effectiveness, Efficiency, and Processes in Brownfield Programming Tasks
Source: arXiv:2506.10051 source file (2025-06-11)
Supplement: Supplementary file 1 [file s8-appendix.tex]

\section{Solutions for Tasks}

\subsection{Add Distance}

\subsubsection{Task 1}
\begin{verbatim}
<div class="mb-3">
    <label for="roundDistance"
        >Distance:<br />
        <input
            class="centered"
            id="roundDistance"
            type="number"
            min="0.01"
            max="62"
            step="0.01"
            required
        />
    </label>
</div>
<div class="mb-3">
    <input
        type="radio"
        id="roundDistanceMiles"
        name="distance"
        value="miles"
        checked
    />
    <label for="miles">Miles</label>
    <input
        type="radio"
        id="roundDistanceKilometers"
        name="distance"
        value="kilometers"
    />
    <label for="kilometers">Kilometers</label><br />
    <div id="roundTimeDescr" class="form-text">
        Enter a distance value between 0.01 and 62
    </div>
</div>
\end{verbatim}

\subsubsection{Task 2}
\begin{verbatim}
const GlobalRoundDistanceMiles = document.getElementById("roundDistanceMiles");
const GlobalRoundDistance = document.getElementById("roundDistance");
const GlobalRoundDistanceKilometers = document.getElementById(
    "roundDistanceKilometers"
);
GlobalRoundDistance.addEventListener("change", function () {
    if (GlobalRoundDistance.value === 0 || GlobalRoundDistance.value === "") {
        GlobalRoundDistanceValue = "";
        return;
    }
    GlobalRoundDistance.value = parseFloat(GlobalRoundDistance.value).toFixed(
        2
    );
    GlobalRoundDistanceMiles.checked
        ? (GlobalRoundDistanceValue = GlobalRoundDistance.value * 5280)
        : (GlobalRoundDistanceValue = GlobalRoundDistance.value * 3280.84);
});
GlobalRoundDistanceMiles.addEventListener("click", updateDistanceUnits);
GlobalRoundDistanceKilometers.addEventListener("click", updateDistanceUnits);
function updateDistanceUnits() {
    if (GlobalRoundDistanceMiles.checked && GlobalRoundDistanceValue !== "") {
        GlobalRoundDistance.value = (
            GlobalRoundDistanceValue * 0.000189394
        ).toFixed(2);
    } else if (GlobalRoundDistanceValue !== "") {
        GlobalRoundDistance.value = (
            GlobalRoundDistanceValue * 0.0003048
        ).toFixed(2);
    }
}
\end{verbatim}

\subsubsection{Task 3}
\begin{verbatim}
// In resetLogRoundForm()
GlobalRoundDistanceValue = "";
GlobalRoundDistance.value = "";
GlobalRoundDistanceMiles.checked = true;
GlobalRoundDistanceKilometers.checked = false;

// In fillRoundForm()
if (round.distance === "") {
    GlobalRoundDistanceValue = "";
    GlobalRoundDistance.value = "";
} else {
    GlobalRoundDistanceValue = round.roundDistance;
    GlobalRoundDistance.value = (round.roundDistance / 5280).toFixed(2);
}

// In Loground()
const newRound = {
    roundDistance: GlobalRoundDistanceValue,
};

// In updateRound()
GlobalUserData.rounds[GlobalRoundIndex].roundDistance =
    GlobalRoundDistanceValue;
\end{verbatim}

\subsection{Add Picture}

\subsubsection{Task 1}
\begin{verbatim}
<div class="mb-3">
    <label for="customPic">
        <input type="checkbox" id="customProfilePicCheck" />
        Use Custom Profile Picture<br />
        <input
            id="customProfilePicPicker"
            type="file"
            class="form-control centered"
            accept=".png, .gif, .jpg"
            aria-describedby="profilePicDescr"
            disabled
        />
    </label>
    <br />
    <img
        id="defaultProfilePicImage"
        src="images/DefaultProfilePic.jpg"
        height="46"
        width="auto"
    />
    <div id="profilePicDescr" class="form-text">
        Check to upload a custom profile picture. Uncheck to use default profile
        picture.
    </div>
</div>
\end{verbatim}

\subsubsection{Task 2}
\begin{verbatim}
const GlobalCustomProfilePicCheck = document.getElementById(
    "customProfilePicCheck"
);
const GlobalCustomProfilePicPicker = document.getElementById(
    "customProfilePicPicker"
);
const GlobalProfilePicImage = document.getElementById("defaultProfilePicImage");

GlobalCustomProfilePicCheck.addEventListener("change", function (e) {
    if (GlobalCustomProfilePicCheck.checked) {
        GlobalCustomProfilePicPicker.disabled = false;
    } else {
        GlobalCustomProfilePicPicker.disabled = true;
        GlobalCustomProfilePicPicker.value = "";
        GlobalProfilePicImage.setAttribute(
            "src",
            "images/DefaultProfilePic.jpg"
        );
    }
});

GlobalCustomProfilePicPicker.addEventListener("change", function (e) {
    if (GlobalCustomProfilePicPicker.value.length !== 0) {
        const reader = new FileReader();
        reader.readAsDataURL(GlobalCustomProfilePicPicker.files[0]);
        reader.addEventListener("load", function () {
            GlobalProfilePicImage.setAttribute("src", this.result);
        });
    }
});
\end{verbatim}

\subsubsection{Task 3}
\begin{verbatim}
// In populateProfileSettingsForm()
if (GlobalUserData.identityInfo.isCustomPic) {
    GlobalCustomProfilePicCheck.checked = true;
    GlobalCustomProfilePicPicker.disabled = false;
    GlobalProfilePicImage.setAttribute(
        "src",
        GlobalUserData.identityInfo.profilePic
    );
} else {
    GlobalCustomProfilePicCheck.checked = false;
    GlobalCustomProfilePicPicker.disabled = true;
    GlobalCustomProfilePicPicker.value = "";
    GlobalProfilePicImage.setAttribute("src", "images/DefaultProfilePic.jpg");
}
// In updateProfile
let image = GlobalProfilePicImage.getAttribute("src");
//inside identityInfo object
isCustomPic: GlobalCustomProfilePicCheck.checked ? true : false,
profilePic: image,
\end{verbatim}
